# Supplementary material for: Phase relations in K_xFe_{2-y}Se_2 and the structure of superconducting K_xFe_2Se_2 via high-resolution synchrotron diffraction
Source: arXiv:1209.1650 source file (2012-09-07)
Supplement: Supplementary file 1 [file shoemaker-sm.pdf]

Phase relations in $K_xFe_{2-y}Se_2$ and the structure of superconducting $K_xFe_2Se_2$ via high-resolution synchrotron diffraction - **Supplemental Material**

D. P. Shoemaker, D. Y. Chung, H. Claus, M. C. Francisco, S. Avci, A. Llobet, and M. G. Kanatzidis

**Contents of this file:**

Rietveld refinement results for APS 11-BM data (pages 1-5)

Single-crystal refinement results (pages 6-8)

Sample numbers correspond to those shown in Figure 10.

**Sample 1 – Powder, non-superconducting**

Nominal composition: $K_{0.8}Fe_{1.6}Se_2$

Synthesis: [$Al_2O_3$ crucible in quartz tube] 4Fe + 5Se 12h ramp to 700ºC 1h hold, 1h cool to room temperature (RT); [$Al_2O_3$ crucible in quartz tube] 2K + $Fe_4Se_5$ 12h ramp to 700ºC, 1h hold, 1h cool to RT; [$Al_2O_3$ crucible in quartz tube] 1h ramp to 700ºC, 1h cool to RT

Phases present: I4/m (100%)

$R_{wp}$ = 0.094, reduced $\chi^2$ = 2.008

I4/m phase: a = 8.721763(10) Å, c = 14.125178(23) Å, stoichiometry: $K_{0.761(5)}Fe_{1.538(4)}Se_2$

| Atom | Site | x | y | z | Uiso*100 (Å$^2$) | Occupancy |
|---|---|---|---|---|---|---|
| K | 8h | 0.1030(5) | 0.7004(6) | 0.5 | 3.33(9) | 0.738(3) |
| K | 2a | 0 | 0 | 0 | 4.54(35) | 0.855(11) |
| Fe | 16i | 0.09242(12) | 0.20069(15) | 0.24697(13) | 1.197(20) | 0.944(2) |
| Fe | 4d | 0.5 | 0 | 0.25 | 1.197(20) | 0.068(3) |
| Se | 16i | 0.10841(11) | 0.70144(14) | 0.14521(4) | 1.760(17) | 1 |
| Se | 4e | 0 | 0 | 0.36030(12) | 1.547(50) | 1 |

**Sample 2 – Crystal, superconducting**

Nominal Composition $K_{0.85}Fe_{1.8}Se_2$

Synthesis: [$Al_2O_3$ crucible in quartz tube] 0.85K + 1.8Fe + 2Se 12h ramp to 600ºC, 4h hold, 4h cool to RT; [$Al_2O_3$ crucible in Nb tube] 50ºC/h ramp to 1050ºC, 2h hold, 5ºC/h cool to 750ºC, 150ºC/h cool to RT, [carbon-coated quartz tube] ~1 second melting of crystals, ice water quench

Phases present: I4/m (100%) (phase separation not resolved due to quenching)

$R_{wp}$ = 0.077, reduced $\chi^2$= 1.038

I4/m phase: a = 8.72201(5) Å, c = 14.12316(10) Å, stoichiometry: $K_{0.817(9)}Fe_{1.545(8)}Se_2$

| Atom | Site | x | y | z | Uiso*100 (Å$^2$) | Occupancy |
|---|---|---|---|---|---|---|
| K | 8h | 0.1207(12) | 0.7066(14) | 0.5 | 3.72(33) | 0.773(7) |
| K | 2a | 0 | 0 | 0 | 3.30(59) | 0.995(19) |
| Fe | 16i | 0.0983(5) | 0.1996(5) | 0.2525(5) | 1.78(4) | 0.878(3) |
| Fe | 4d | 0.5 | 0 | 0.25 | 1.78(4) | 0.351(7) |
| Se | 16i | 0.1068(4) | 0.6988(4) | 0.14334(10) | 2.46(5) | 1 |
| Se | 4e | 0 | 0 | 0.35340(34) | 2.12(13) | 1 |

**Sample 3 – Crystal, superconducting**

Nominal Composition $K_{0.85}Fe_{1.9}Se_2$

Synthesis: [$Al_2O_3$ crucible in quartz tube] 0.85K + 1.9Fe + 2Se 12h ramp to 650ºC, 4h hold, 4h cool to RT; [$Al_2O_3$ crucible in Nb tube] 50ºC/h ramp to 1050ºC, 2h hold, 6ºC/h cool to 750ºC, 100ºC/h cool to RT

Phases present: I4/m (82 wt%), I4/mmm (12 wt%)

$R_{wp}$ = 0.0973, reduced $\chi^2$= 1.988

I4/m phase: a = 8.72481(7) Å, c = 14.11933(13) Å, stoichiometry: $K_{0.76(1)}Fe_{1.487(8)}Se_2$

| Atom | Site | x | y | z | Uiso*100 (Å$^2$) | Occupancy |
|---|---|---|---|---|---|---|
| K | 8h | 0.1168(17) | 0.7176(15) | 0.5 | 1.64(31) | 0.760(8) |
| K | 2a | 0 | 0 | 0 | 2.60(35) | 0.766(21) |
| Fe | 16i | 0.1002(5) | 0.1933(6) | 0.24582(31) | 1.21(6) | 0.851(3) |
| Fe | 4d | 0.5 | 0 | 0.25 | 1.21(6) | 0.314(9) |
| Se | 16i | 0.1043(5) | 0.6976(5) | 0.14558(12) | 2.50(6) | 1 |
| Se | 4e | 0 | 0 | 0.36138(45) | 1.56(20) | 1 |

I4/mmm phase: a = 3.83414(20), Å c = 14.2360(12) Å, stoichiometry: $K_{0.58(2)}Fe_{0.92(2)}Se_2$

| Atom | Site | x | y | z | Uiso*100 (Å$^2$) | Occupancy |
|---|---|---|---|---|---|---|
| K | 2a | 0 | 0 | 0 | 3.7(8) | 0.583(23) |
| Fe | 4d | 0 | 0.5 | 0.25 | 1.03(22) | 0.920(15) |
| Se | 4e | 0 | 0 | 0.357567 | 2.56(18) | 1 |

**Sample 4 – Crystal, superconducting**

Nominal Composition $K_{0.85}Fe_{1.9}Se_2$

Synthesis: [$Al_2O_3$ crucible in quartz tube] 0.85K + 1.9Fe + 2Se 12h ramp to 600ºC, 4h hold, 4h cool to RT; [$Al_2O_3$ crucible in Nb tube] 50ºC/h ramp to 1100ºC, 2h hold, 5ºC/h cool to 750ºC, 150ºC/h cool to RT

Phases present: I4/m (81 wt%), I4/mmm (18 wt%), Fe (1 wt%)

$R_{wp}$ = 0.0986, reduced $\chi^2$= 1.809

I4/m phase: a = 8.72659(11), Å c = 14.11929(23) Å, stoichiometry: $K_{0.80(2)}Fe_{1.44(2)}Se_2$

| Atom | Site | x | y | z | Uiso*100 (Å$^2$) | Occupancy |
|---|---|---|---|---|---|---|
| K | 8h | 0.1185(29) | 0.7112(34) | 0.5 | 3.34(30) | 0.746(10) |
| K | 2a | 0 | 0 | 0 | 3.34(30) | 1.030(36) |
| Fe | 16i | 0.1037(10) | 0.1946(10) | 0.2577(4) | 0.48(9) | 0.801(6) |
| Fe | 4d | 0.5 | 0 | 0.25 | 0.48(9) | 0.397(16) |
| Se | 16i | 0.1026(8) | 0.7042(8) | 0.14527(17) | 1.98(10) | 1 |
| Se | 4e | 0 | 0 | 0.36404(58) | 1.54(35) | 1 |

I4/mmm phase: a = 3.82803(23), Å c = 14.2634(10) Å, stoichiometry: $K_{0.545(14)}Fe_{1.00(1)}Se_2$

| Atom | Site | x | y | z | Uiso*100 (Å$^2$) | Occupancy |
|---|---|---|---|---|---|---|
| K | 2a | 0 | 0 | 0 | 2 | 0.545(14) |
| Fe | 4d | 0 | 0.5 | 0.25 | 2 | 1.001(11) |
| Se | 4e | 0 | 0 | 0.35773(33) | 1.82(18) | 1 |

**Sample 5 – Crystal, superconducting**

Nominal Composition $K_{0.85}Fe_{1.9}Se_2$

Synthesis: [$Al_2O_3$ crucible in quartz tube] 0.85K + 1.9Fe + 2Se 12h ramp to 600ºC, 4h hold, 4h cool to RT; [$Al_2O_3$ crucible in Nb tube] 50ºC/h ramp to 1100ºC, 2h hold, 5ºC/h cool to 750ºC, 150ºC/h cool to RT; [carbon-coated quartz tube] ~1 second melting of crystals, ice water quench

Phases present: I4/m (100%) (phase separation not resolved due to quenching)

$R_{wp}$ = 0.1045, reduced $\chi^2$= 1.293

I4/m phase: a = 8.72711(10), Å c = 14.12185(14) Å, stoichiometry: $K_{0.77(1)}Fe_{1.66(1)}Se_2$

| Atom | Site | x | y | z | Uiso*100 (Å$^2$) | Occupancy |
|---|---|---|---|---|---|---|
| K | 8h | 0.1269(14) | 0.7137(18) | 0.5 | 1.1(4) | 0.739(9) |
| K | 2a | 0 | 0 | 0 | 0.9(9) | 0.891(29) |
| Fe | 16i | 0.1091(6) | 0.1922(7) | 0.2532(5) | 2.00(13) | 0.869(4) |
| Fe | 4d | 0.5 | 0 | 0.25 | 2.37(63) | 0.664(11) |
| Se | 16i | 0.1035(5) | 0.7089(5) | 0.14629(15) | 2.04(8) | 1 |
| Se | 4e | 0 | 0 | 0.36015(48) | 1.06(23) | 1 |

**Sample 6 – Crystal, superconducting**

Nominal Composition $K_{0.85}Fe_{1.9}Se_2$

Synthesis: [$Al_2O_3$ crucible in quartz tube] 0.85K + 1.9Fe + 2Se 12h ramp to 600ºC, 4h hold, 4h cool to RT; [$Al_2O_3$ crucible in Nb tube] 50ºC/h ramp to 1100ºC, 2h hold, 5ºC/h cool to 750ºC, 150ºC/h cool to RT

Phases present: I4/m (85 wt%), I4/mmm (13 wt%), Fe (2 wt %)

$R_{wp}$ = 0.0741, reduced $\chi^2$= 2.12

I4/m phase: a = 8.72950(9), Å c = 14.11085(19) Å, stoichiometry: $K_{0.88(1)}Fe_{1.455(8)}Se_2$

| Atom | Site | x | y | z | Uiso*100 (Å$^2$) | Occupancy |
|---|---|---|---|---|---|---|
| K | 8h | 0.1152(16) | 0.7220(16) | 0.5 | 5.1(5) | 0.855(9) |
| K | 2a | 0 | 0 | 0 | 2.1(7) | 0.967(25) |
| Fe | 16i | 0.1008(6) | 0.2022(6) | 0.2555(4) | 0.78(6) | 0.826(3) |
| Fe | 4d | 0.5 | 0 | 0.25 | 0.78(6) | 0.333(9) |
| Se | 16i | 0.1026(5) | 0.7010(5) | 0.14224(14) | 2.24(9) | 1 |
| Se | 4e | 0 | 0 | 0.35312(52) | 0.89(26) | 1 |

I4/mmm phase: a = 3.82707(26), Å c = 14.2658(15) Å, stoichiometry: $K_{0.38(2)}Fe_{1.03(1)}Se_2$

| Atom | Site | x | y | z | Uiso*100 (Å$^2$) | Occupancy |
|---|---|---|---|---|---|---|
| K | 2a | 0 | 0 | 0 | 2.2(14) | 0.376(19) |
| Fe | 4d | 0 | 0.5 | 0.25 | 3.11(31) | 1.033(14) |
| Se | 4e | 0 | 0 | 0.35630(33) | 3.22(19) | 1 |

**Sample 7 – Crystal, non-superconducting**

Nominal Composition $K_{0.8}Fe_2Se_2$

Synthesis: [$Al_2O_3$ crucible in quartz tube] Fe + Se 12h ramp to 600ºC, 4h hold, 4h cool to RT; [$Al_2O_3$ crucible in quartz tube] 0.8K + 2FeSe 12h ramp to 600ºC, 4h hold, 4h cool to RT; [quartz tube] Bridgman growth at 960ºC with 5mm/h dropping rate

Phases present: I4/m (92 wt%), I4/mmm** (8 wt%), Fe (0.3 wt%)

$R_{wp}$ = 0.0805, reduced $\chi^2$= 2.339

I4/m phase: a = 8.73198(4), Å c = 14.10359(9) Å, stoichiometry: $K_{0.805(8)}Fe_{1.493(6)}Se_2$

| Atom | Site | x | y | z | Uiso*100 (Å$^2$) | Occupancy |
|---|---|---|---|---|---|---|
| K | 8h | 0.1129(12) | 0.7192(13) | 0.5 | 2.10(23) | 0.781(6) |
| K | 2a | 0 | 0 | 0 | 3.07(25) | 0.902(17) |
| Fe | 16i | 0.0987(4) | 0.1987(4) | 0.25456(26) | 0.90(4) | 0.845(2) |
| Fe | 4d | 0.5 | 0 | 0.25 | 0.90(4) | 0.353(6) |
| Se | 16i | 0.10279(34) | 0.70505(30) | 0.14468(8) | 2.43(4) | 1 |
| Se | 4e | 0 | 0 | 0.35927(30) | 1.13(13) | 1 |

**The refined lattice parameters for this phase are distinct from the I4/mmm phase found in superconducting samples: a=3.8641(2) Å and c = 14.3678(8) Å.

**Sample 8 – Crystal, non-superconducting**

Nominal Composition $K_{0.8}Fe_{1.6}Se_2$

Synthesis: [$Al_2O_3$ crucible in quartz tube] 1.6Fe + 2Se 12h ramp to 600ºC, 4h hold, 4h cool to RT; [$Al_2O_3$ crucible in quartz tube] 0.8K + $Fe_{1.6}Se_2$ 12h ramp to 600ºC, 4h hold, 4h cool to RT; [Al2O3 crucible in Nb tube] 50ºC/h ramp to 1100ºC, 2h hold, 5ºC/h cool to 750ºC, 150ºC/h cool to RT

Phases present: I4/m (100%)

$R_{wp}$ = 0.1096, reduced $\chi^2$ = 2.324

I4/m phase: a = 8.74536(8), Å c = 14.10024(18) Å, stoichiometry: $K_{0.837(9)}Fe_{1.435(8)}Se_2$

| Atom | Site | x | y | z | Uiso*100 (Å$^2$) | Occupancy |
|---|---|---|---|---|---|---|
| K | 8h | 0.1159(15) | 0.7259(13) | 0.5 | 4.28(23) | 0.806(7) |
| K | 2a | 0 | 0 | 0 | 4.28(23) | 0.959(18) |
| Fe | 16i | 0.1023(6) | 0.2068(6) | 0.25666(30) | 1.13(7) | 0.819(3) |
| Fe | 4d | 0.5 | 0 | 0.25 | 1.13(7) | 0.312(8) |
| Se | 16i | 0.0997(5) | 0.7045(4) | 0.14146(11) | 2.34(7) | 1 |
| Se | 4e | 0 | 0 | 0.35030(39) | 0.64(17) | 1 |

**Sample 9 – Crystal, non-superconducting**
Nominal Composition $K_{0.85}Fe_{1.9}Se_2$
Synthesis: [$Al_2O_3$ crucible in quartz tube] 0.85K + 1.9Fe + 2Se 50ºC/h ramp to 1050ºC, 2h hold, 6ºC/h cool to 750ºC, 100ºC/h cool to RT
Phases present: I4/m (100%)
$R_{wp}$ = 0.0812, reduced $\chi 2$ = 1.532
I4/m phase: a = 8.746631(29), Å c = 14.06401(6) Å, stoichiometry: $K_{0.838(8)}Fe_{1.606(5)}Se_2$

| Atom | Site | x | y | z | Uiso*100 (Å$^2$) | Occupancy |
|---|---|---|---|---|---|---|
| K | 8h | 0.1131(8) | 0.7092(9) | 0.5 | 3.17(15) | 0.799(5) |
| K | 2a | 0 | 0 | 0 | 3.68(63) | 0.993(18) |
| Fe | 16i | 0.09812(30) | 0.19815(34) | 0.25057(31) | 1.881(29) | 0.903(2) |
| Fe | 4d | 0.5 | 0 | 0.25 | 1.881(29) | 0.403(5) |
| Se | 16i | 0.10587(26) | 0.70437(27) | 0.14400(8) | 1.96(4) | 1 |
| Se | 4e | 0 | 0 | 0.35805(26) | 1.50(10) | 1 |

**$KFe_{1.6}Se_2$ – Powder, non-superconducting**
Nominal Composition $KFe_{1.5}Se_2$
Synthesis: [$Al_2O_3$ crucible in quartz tube] 1.5Fe + 2Se 12h ramp to 700ºC 1h hold, 1h cool to RT; [$Al_2O_3$ crucible in quartz tube] K + $Fe_{1.5}Se_2$ 12h ramp to 700ºC, 1h hold, 1h cool to RT; [$Al_2O_3$ crucible in quartz tube] 1h ramp to 700ºC, 1h cool to RT
Phases present: I4/mmm
$R_{wp}$ = 0.1366, reduced $\chi 2$ = 2.16
I4/mmm phase: a = 3.952954(7), Å c = 13.86531(3) Å, stoichiometry: $K_{0.949(4)}Fe_{1.606(6)}Se_2$

| Atom | Site | x | y | z | $U_{11}$=$U_{22}$*100 (Å$^2$) | $U_{33}$*100 (Å$^2$) | Occupancy |
|---|---|---|---|---|---|---|---|
| K | 2a | 0 | 0 | 0 | 1.81(8) | 1.34(11) | 0.959(4) |
| Fe | 4d | 0 | 0.5 | 0.25 | 2.16(5) | 1.27(7) | 0.803(3) |
| Se | 4e | 0 | 0 | 0.35674(4) | 1.359(22) | 2.27(4) | 1 |

**Single-crystal refinement: Sample 8 – Crystal, non-superconducting, 293 K**

| | |
|---|---|
| Refined formula | $K_{0.793(14)}Fe_{1.562(10)}Se_2$ |
| Wavelength | 0.71073 Å |
| Space group | *I*4/*m* (87) |
| Unit cell dimensions | a = 8.7313(12) Å, α = 90.00°<br>b = 8.7313(12) Å, β = 90.00°<br>c = 14.062(3) Å, γ = 90.00° |
| Volume | 1072.0(3) Å$^3$ |
| Z | 4 |
| Density (calculated) | 4.315 g/cm$^3$ |
| Absorption coefficient | 22.988 mm$^{-1}$ |
| Crystal size | 0.31 x 0.20 x 0.09 mm$^3$ |
| F(000) | 1248 |
| θ range for data collection | 5.42 to 26.32° |
| Index ranges | -10<=h<=10, -10<=k<=10, -17<=l<=17 |
| Reflections collected | 3883 |
| Independent reflections | 573 [$R_{int}$ = 0.0812] |
| Completeness to θ = 26.32° | 99% |
| Refinement method | Full-matrix least-squares on $F^2$ |
| Data / restraints / parameters | 573 / 0 / 37 |
| Goodness-of-fit | 0.960 |
| Final R indices [>2σ(I)] | $R_{obs}$ = 0.0388, $wR_{obs}$ = 0.0769 |
| R indices [all data] | $R_{all}$ = 0.0517, $wR_{all}$ = 0.0818 |
| Largest diff. peak and hole | 2.386 and -0.870 e· Å$^{-3}$ |

$R = \Sigma||F_o|-|F_c|| / \Sigma|F_o|$, $wR = \{\Sigma[w(|F_o|^2 - |F_c|^2)^2] / \Sigma[w(|F_o|^4)]\}^{1/2}$

$w=1/[\sigma^2(Fo^2)+(0.0433P)^2+0.0000P]$ where $P=(Fo^2+2Fc^2)/3$

Atomic coordinates (x10$^4$) and equivalent isotropic displacement parameters (Å$^2$x10$^3$)

| Label | x | y | z | Occupancy | $U_{eq}$* |
|---|---|---|---|---|---|
| Se(1) | 1083(1) | 7004(1) | 1452(1) | 1 | 19(1) |
| Se(2) | 0 | 0 | 3607(1) | 1 | 18(1) |
| Fe(3) | 930(1) | 1989(1) | 2473(1) | 0.925(4) | 17(1) |
| Fe(4) | 5000 | 0 | 2500 | 0.205(8) | 14(2) |
| K(5) | 979(2) | 6943(2) | 5000 | 0.782(13) | 34(1) |
| K(6) | 0 | 0 | 0 | 0.838(18) | 36(2) |

*$U_{eq}$ is defined as one third of the trace of the orthogonalized $U_{ij}$ tensor.

Anisotropic displacement parameters (Å$^2$x10$^3$)

| Label | $U_{11}$ | $U_{22}$ | $U_{33}$ | $U_{12}$ | $U_{13}$ | $U_{23}$ |
|---|---|---|---|---|---|---|
| Se(1) | 17(1) | 17(1) | 23(1) | 2(1) | -1(1) | -3(1) |
| Se(2) | 15(1) | 15(1) | 23(1) | 0 | 0 | 0 |
| Fe(3) | 14(1) | 15(1) | 22(1) | 0(1) | 1(1) | 0(1) |
| Fe(4) | 11(3) | 11(3) | 19(4) | 0 | 0 | 0 |
| K(5) | 33(2) | 41(2) | 26(2) | 2(1) | 0 | 0 |
| K(6) | 41(2) | 41(2) | 25(2) | 0 | 0 | 0 |

The anisotropic displacement factor exponent takes the form: $-2\pi^2[h^2a^{*2}U_{11} + ... + 2hka^*b^*U_{12}]$.

**Single-crystal refinement: Sample 4 – Crystal, superconducting, 293 K**

| | |
|---|---|
| Refined formula | $K_{0.723(16)}Fe_{1.631(12)}Se_2$ |
| Wavelength | 0.71073 Å |
| Space group | *I*4/*m* (87) |
| Unit cell dimensions | a = 8.6868(12) Å, α = 90.00°<br>b = 8.6868(12) Å, β = 90.00°<br>c = 14.127(3) Å, γ = 90.00° |
| Volume | 1066.0(3) $Å^3$ |
| Z | 4 |
| Density (calculated) | 4.339 $g/cm^3$ |
| Absorption coefficient | 23.118 $mm^{-1}$ |
| Crystal size | 0.31 x 0.16 x 0.09 $mm^3$ |
| F(000) | 1248 |
| θ range for data collection | 5.44 to 26.36° |
| Index ranges | -10<=h<=10, -10<=k<=10, -17<=l<=17 |
| Reflections collected | 3902 |
| Independent reflections | 571 [$R_{int}$ = 0.1177] |
| Completeness to θ = 26.36° | 99% |
| Refinement method | Full-matrix least-squares on $F^2$ |
| Data / restraints / parameters | 571 / 0 / 36 |
| Goodness-of-fit | 0.977 |
| Final R indices [>2σ(I)] | $R_{obs}$ = 0.0504, $wR_{obs}$ = 0.1087 |
| R indices [all data] | $R_{all}$ = 0.0746, $wR_{all}$ = 0.1232 |
| Largest diff. peak and hole | 1.511 and -0.895 e·$Å^{-3}$ |

$R = \Sigma||F_o|-|F_c|| / \Sigma|F_o|$, $wR = \{\Sigma[w(|F_o|^2 - |F_c|^2)^2] / \Sigma[w(|F_o|^4)]\}^{1/2}$ and calc $w=1/[\sigma^2(Fo^2)+(0.0530P)^2+0.0000P]$ where $P=(Fo^2+2Fc^2)/3$

Atomic coordinates ($x10^4$) and equivalent isotropic displacement parameters ($Å^2x10^3$)

| Label | x | y | z | Occupancy | $U_{eq}$* |
|---|---|---|---|---|---|
| Se(1) | 1067(1) | 7001(1) | 1449(1) | 1 | 40(1) |
| Se(2) | 0 | 0 | 3596(1) | 1 | 39(1) |
| Fe(3) | 942(1) | 1994(1) | 2479(1) | 0.923(5) | 38(1) |
| Fe(4) | 5000 | 0 | 2500 | 0.386(9) | 45(2) |
| K(5) | 980(3) | 6951(3) | 5000 | 0.719(15) | 52(2) |
| K(6) | 0 | 0 | 0 | 0.74(2) | 54(2) |

*$U_{eq}$ is defined as one third of the trace of the orthogonalized $U_{ij}$ tensor.

Anisotropic displacement parameters ($Å^2x10^3$)

| Label | $U_{11}$ | $U_{22}$ | $U_{33}$ | $U_{12}$ | $U_{13}$ | $U_{23}$ |
|---|---|---|---|---|---|---|
| Se(1) | 40(1) | 39(1) | 41(1) | 1(1) | 0(1) | -2(1) |
| Se(2) | 38(1) | 38(1) | 41(1) | 0 | 0 | 0 |
| Fe(3) | 36(1) | 38(1) | 41(1) | 0(1) | 2(1) | 0(1) |
| Fe(4) | 47(2) | 47(2) | 40(3) | 0 | 0 | 0 |
| K(5) | 53(2) | 62(2) | 43(2) | 2(2) | 0 | 0 |
| K(6) | 58(3) | 58(3) | 46(4) | 0 | 0 | 0 |

The anisotropic displacement factor exponent takes the form: $-2\pi^2[h^2a^{*2}U_{11} + ... + 2hka^*b^*U_{12}]$.

**Single-crystal refinement: Oxidized phase: non-superconducting sample 8 after air exposure**

| | |
|---|---|
| Refined formula | $K_{0.51(5)}Fe_{0.698(19)}Se$ |
| Temperature | 293(2) K |
| Wavelength | 0.71073 Å |
| Space group | *P*4/*nmm* (129) |
| Unit cell dimensions | a = 3.8952(6) Å, α = 90.00°<br>b = 3.8952(6) Å, β = 90.00°<br>c = 9.1948(18) Å, γ = 90.00° |
| Volume | 139.51(4) Å$^3$ |
| Z | 2 |
| Density (calculated) | 7.824 g/cm$^3$ |
| Absorption coefficient | 43.409 mm$^{-1}$ |
| Crystal size | 0.34 x 0.33 x 0.12 mm$^3$ |
| F(000) | 293 |
| θ range for data collection | 2.21 to 24.63° |
| Index ranges | -4<=h<=4, -4<=k<=4, -10<=l<=9 |
| Reflections collected | 830 |
| Independent reflections | 99 [$R_{int}$ = 0.1807] |
| Completeness to θ = 24.63° | 100% |
| Refinement method | Full-matrix least-squares on $F^2$ |
| Data / restraints / parameters | 99 / 0 / 12 |
| Goodness-of-fit | 0.849 |
| Final R indices [>2σ(I)] | $R_{obs}$ = 0.0653, $wR_{obs}$ = 0.1355 |
| R indices [all data] | $R_{all}$ = 0.1036, $wR_{all}$ = 0.1541 |
| Largest diff. peak and hole | 1.085 and -0.825 e·Å$^{-3}$ |

$R = \Sigma||F_o|-|F_c|| / \Sigma|F_o|$, $wR = \{\Sigma[w(|F_o|^2 - |F_c|^2)^2] / \Sigma[w(|F_o|^4)]\}^{1/2}$
$w=1/[\sigma^2(Fo^2)+(0.1000P)^2+0.0000P]$ where $P=(Fo^2+2Fc^2)/3$

Atomic coordinates (x10$^4$) and equivalent isotropic displacement parameters (Å$^2$x10$^3$)

| Label | x | y | z | Occupancy | $U_{eq}$* |
|---|---|---|---|---|---|
| Se(1) | 2500 | 2500 | 1559(6) | 1 | 79(2) |
| Fe(2) | 7500 | 2500 | 0 | 0.698(19) | 70(3) |
| K(1) | 7500 | 7500 | 4280(40) | 0.51(5) | 142(16) |

*$U_{eq}$ is defined as one third of the trace of the orthogonalized $U_{ij}$ tensor.

Anisotropic displacement parameters (Å$^2$x10$^3$)

| Label | $U_{11}$ | $U_{22}$ | $U_{33}$ | $U_{12}$ | $U_{13}$ | $U_{23}$ |
|---|---|---|---|---|---|---|
| Se(1) | 61(2) | 61(2) | 116(4) | 0 | 0 | 0 |
| Fe(2) | 45(3) | 45(3) | 120(8) | 0 | 0 | 0 |
| K(1) | 140(19) | 140(19) | 150(20) | 0 | 0 | 0 |

The anisotropic displacement factor exponent takes the form: $-2\pi^2[h^2a^{*2}U_{11} + ... + 2hka^*b^*U_{12}]$.
